# Supplementary material for: PIONEER: Studies of Rare Pion Decays
Source: arXiv:2203.01981 source file (2022-03-08)
Supplement: Supplementary file 2 [file inTargetDifSuppression.tex]

\section{In-target Decay-in-flight $\pi \rightarrow \mu \nu$ Suppression with BDT}
\label{sec:DIFsuppression_BDT_appendix}

\begin{itemize}
    \item plots of input features (pienu vs DIF)
    \item BDT score distribution
    \item ROC curve
    \item suppression factor with the consideration of energy smearing
\end{itemize}
