# Supplementary material for: PIONEER: Studies of Rare Pion Decays
Source: arXiv:2203.01981 source file (2022-03-08)
Supplement: Supplementary file 3 [file ATAR_appendix.tex]

\section{ATAR technical details}
\label{sec:ATAR_appendix}

%ATAR Technical Details

As introduced in Sec.~\ref{sec:ATAR}, the highly segmented active target (ATAR) is a key new feature of the proposed PIONEER experiment which will define the fiducial pion stop region, provide high resolution timing information, and furnish selective event triggers. Advanced technical details and studies will be covered by this Appendix. 

A brief summary of the baseline ATAR design follows. 
The ATAR tentative design dimensions are 2 $\times$ 2\,cm$^2$ transverse to the beam, in the beam direction individual silicon sensors are tightly stacked with a total thickness of roughly 6\,mm. 
Planes of the ATAR are composed of LGAD sensors, for which a thickness of 120\,$\mu$m and a strip geometry with a pitch of 200\,$\mu$m is foreseen. 
The detectors are paired with the high-voltage facing each other to avoid ground and high voltage in proximity. These strip sensor pairs are oriented at 90$\degree$ to each other in subsequent staggered planes to provide measurement of both coordinates of interest and allow space for the readout and wirebonds.
% the electronic readout is placed outside of the active region and connected through a short flex.
In the preliminary design, the strips are wire bonded to a flex, alternating the connection on the four sides of the ATAR, that brings the signal to a readout chip.
This positions the chip a few cm away from the active volume and outside of the path of the exiting positrons, reducing the degradation of their energy resolution.
The readout ASIC sits on the first flex that tapers out to accommodate the additional traces. Then this flex is connected, via connector, to a PCB connected to a second flex that brings the amplified signal to the digitizers in the back end. 
A schematic drawing of the ATAR is shown in  Sec.~\ref{sec:ATAR}, Fig.~\ref{fig:ATAR_scheme}.

\subsection{LGAD technology}
\label{sec:LGAD_app}

The chosen technology for the ATAR is based on  Low Gain Avalanche Detectors (LGAD) \cite{bib:LGAD}, thin silicon detectors with moderate internal gain. LGADs are composed by a low doped region referred to as `bulk', typically 50\,$\mu$m thick, and a highly doped thin region, a few $\mu$m from the electrodes, called `gain layer'. The electric field in the gain layer is high enough to generate charge multiplication from electrons but not from holes: this mechanism allows to have moderate charge multiplication (up to 50) without generating an avalanche. A schematic cross-section of an LGAD can be found in Fig.~\ref{fig:Pulse} (Left). Due to the internal gain and thin bulk, LGADs have fast rise time and short full charge collection time.

\begin{figure}[htbp]
\centering
\includegraphics[width=0.45\textwidth]{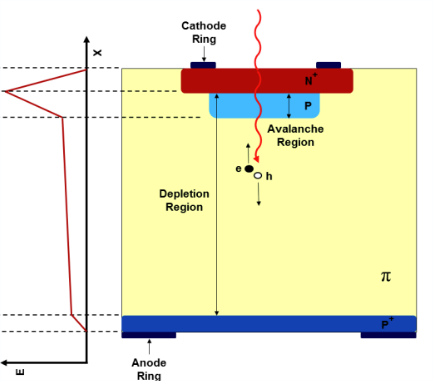}
\includegraphics[width=0.54\textwidth]{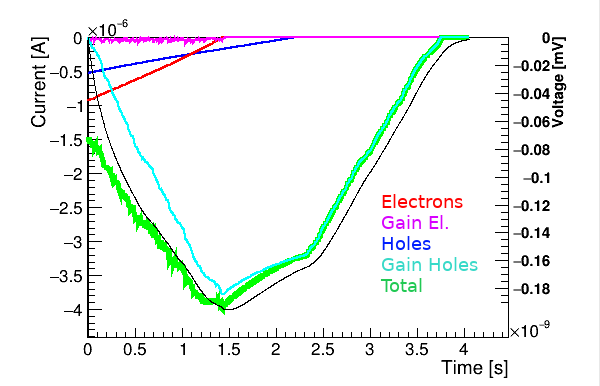}
\caption{Left: LGAD schematic cross-section with electric field on the left. Right: Simulated pulse shape for a MIP in a 120~$\mu$m thick LGAD (Weightfield2 \cite{WF2}). The black line is the response of a 2\,GHz bandwidth electronic readout.}
\label{fig:Pulse}
\end{figure}

The best estimate at present for the sensor thickness is around 120\,$\mu$m to avoid support structures for the sensor, which would introduce dead areas and inactive material within the beam. Normally LGADs have a thickness of 50\,$\mu$m or less, so the exact sensor performance of a non-conventional 120\,$\mu$m-thick LGAD will need to be established by tests on more mature prototypes.
Using fast electronics is expected to result in a pulse rise time of about 1\,ns for an LGAD of this thickness, as shown in Fig.~\ref{fig:Pulse} (Right). The time resolution on the rising edge should be less than 100\,ps for a minimum ionizing signal, down to much better time resolution for large $\pi/\mu$ signals.
Such a sensor would be able to separate two closely overlapping hits if they arrive more than 1.5\,ns apart.

The LGAD technology was chosen over standard Silicon technology because of the intrinsic gain and thin bulk. 
Normal silicon detectors without gain need 300--500\,$\mu$m of active silicon to have enough collected charge for high MIP detection efficiency (unless for the case of very small pixels, where a lower capacitance and noise allows 150\,$\mu$m of thickness).
This would reduce the achievable granularity in the direction of the beam and increase significantly the pulse width and therefore reduce the temporal pulse separation discrimination.
The increased S/N of LGADs is also helpful for signal transmission through the first flex to the  ASIC.

HV-CMOS was also considered as a possibility, however monolithic pixels usually have non-depleted regions between pixels, and furthermore to achieve the same level of time resolution, the power would need to be increased to a level that is not sustainable for the ATAR. 
If the amplifier chip is removed from the compact region of the ATAR as in the case of the current design, heat dissipation from the readout electronics is less problematic.
3D sensors have a similar issue of non-depleted regions, furthermore the temporal pulse separation discrimination would be depending on the strip pitch.
On top of this, LGADs can be produced by several small and research foundries in addition to commercial vendors, making the prototyping phase easier and reducing the risk of production delays in case of large-scale availability bottlenecks at big companies. 

Current standard LGADs are limited in terms of granularity and active area due to a protection structure (junction termination extension) at the edge of the high field area of the gain layer, necessary to avoid breakdown of the sensor.
A typical width for such an inter-pad gap in an LGAD is around 50--100\,$\mu$m, and thus limits the granularity to the mm scale for regular LGADs.
To achieve a ~100\% active area, several technologies still at prototype level are being evaluated for PIONEER, such as AC-LGADs~\cite{Apresyan:2020ipp} (studies shown in Appendix~\ref{sec:ACLGAD_app}), TI-LGADs~\cite{9081916} (studies shown in Appendix~\ref{sec:TILGAD_app}) and DJ-LGAD~\cite{Ayyoub:2021dgk}.
The DJ-LGAD is the newest high-granularity design and no prototype exists at the moment, however a prototype run is expected to be finished and tested by Q1 2022.

Radiation damage is not expected to be an issue for the initial phases of \nexp. For the \pie~ phase a total fluence of $10^{13}$ is expected, this is at an order of magnitude away from where radiation damage would significantly degrade the performance of LGADs~\cite{CERN-LHCC-2020-007}.
However $10^7$ pions per second are expected in the pion beta decay phase, this adds up to $10^{14}$ for a full year of data taking.
The integrated radiation damage of several $10^{14}$ for the full run will start to affect LGADs performance~\cite{CERN-LHCC-2020-007}, although the fluence is still moderate in comparison to other LGAD applications.
A simple solution to reduce the radiation damage is the substitution of the ATAR at the mid-life of the experiment. 

%%%%%%%%%%%%%%%%%%%%%%%%%%%%%%%%%%%%%%%%%%%%%%%%%%%%%%%%%%%%

\subsection{AC-LGAD preliminary studies}
\label{sec:ACLGAD_app}

AC-LGADs overcome the granularity limitation of traditional LGADs and have been shown to provide spatial resolution of the order of tens of $\mu$m~\cite{Tornago:2020otn}. This remarkable feature is achieved with an unsegmented (p-type) gain layer and a resistive (n-type) N-layer. An insulating dielectric layer separates the metal readout pads from the N+ resistive layer. This design also allows to have a completely active sensor with no dead regions.
AC-LGADs have intrinsic charge sharing between AC metal pads, so the signal can be picked up by multiple channels at the same time.
In a low hit-density environment, such as PIONEER, this allows to have a sparse electrode distribution but with elevated position resolution together with a 100\% active area.
Charge depositions can be then reconstructed by calculating the fraction of signal present in all nearby electrodes. With a strip geometry, the hit reconstruction can be made using two neighboring strips.

The following studies were conducted on strip AC-LGAD prototypes from Brookhaven National Lab (BNL) (Fig.~\ref{fig:FNAL_data}, Left). 
The sensors have been tested with a laboratory IR laser TCT station~\cite{Particulars} and at a Fermilab (FNAL) test beam~\cite{ACLGADpico}.
In both setups the sensors are mounted on fast analog amplifier boards (16 channels) with 1\,GHz of bandwidth (designed at FNAL), the board is read out by a fast oscilloscope (2\,GHz, 20Gs).
The response of two strips of a 200\,$\mu$m pitch BNL AC-LGAD as a function of position can be seen in Fig.~\ref{fig:FNAL_data} (Right).

\begin{figure}[htbp]
\centering
\includegraphics[width=0.4\textwidth]{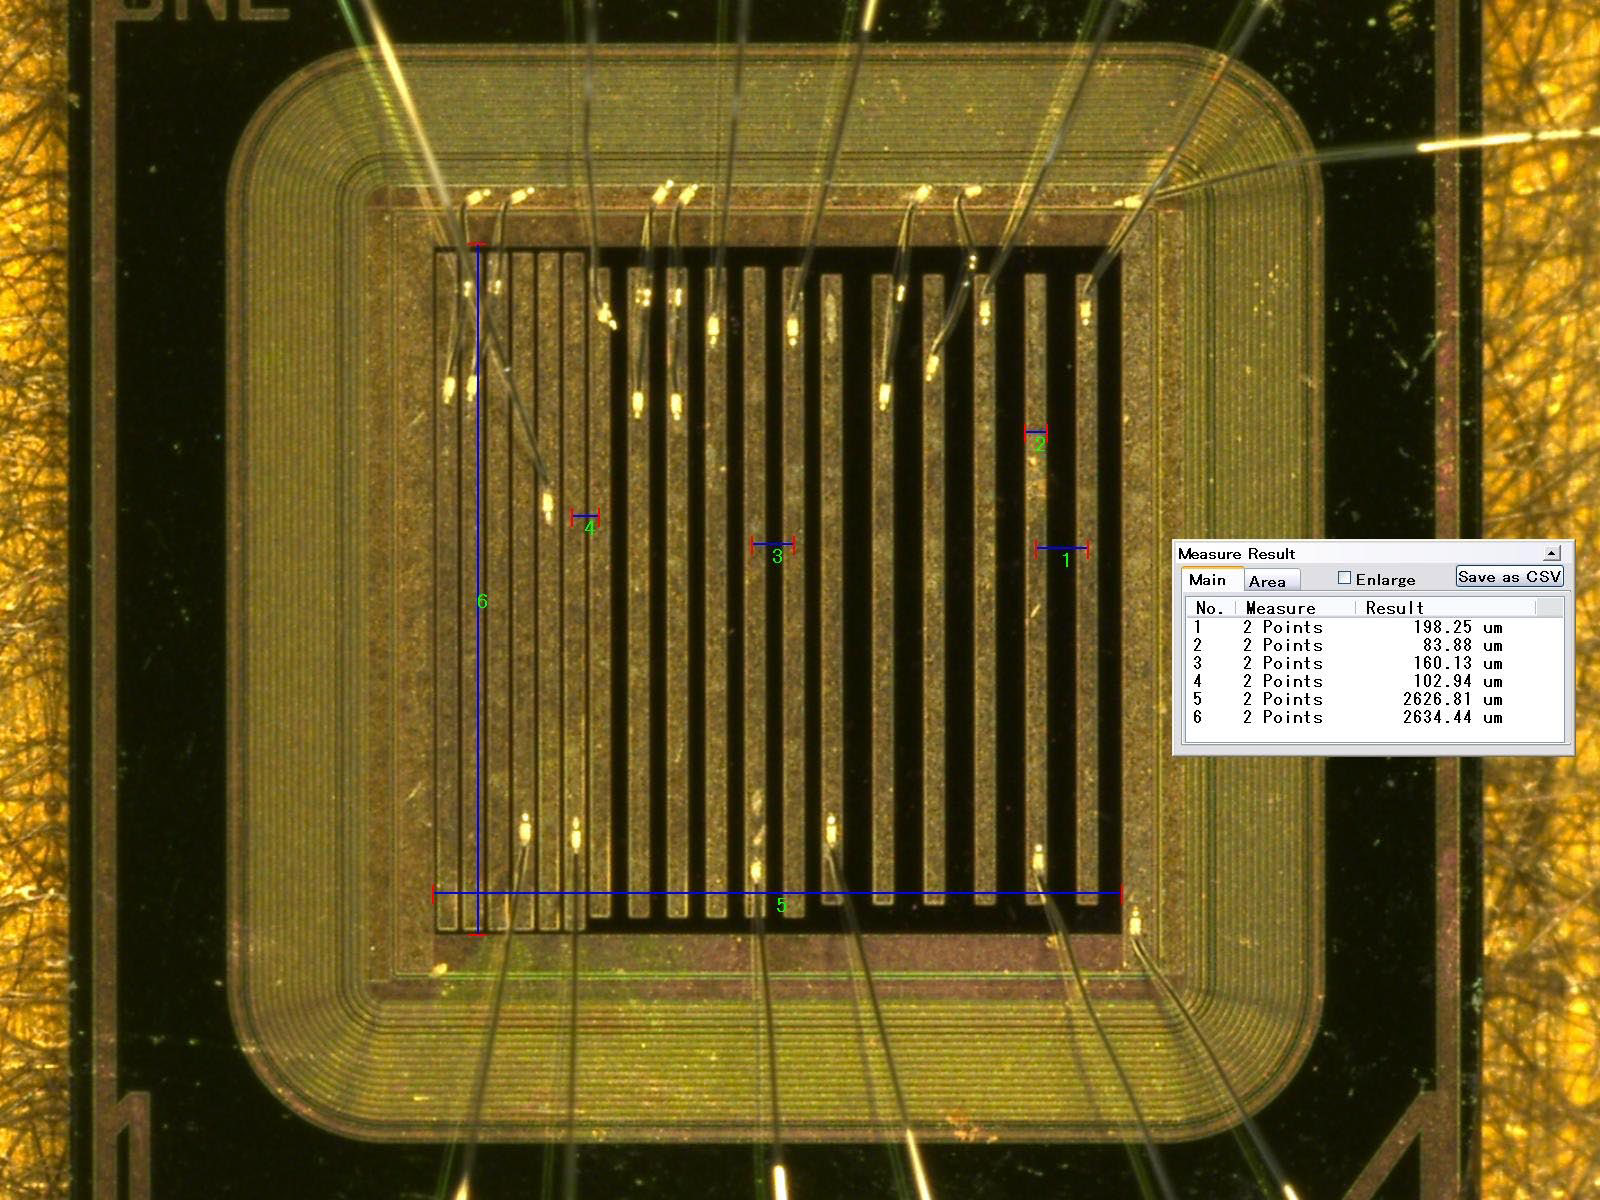}
\includegraphics[width=0.5\textwidth]{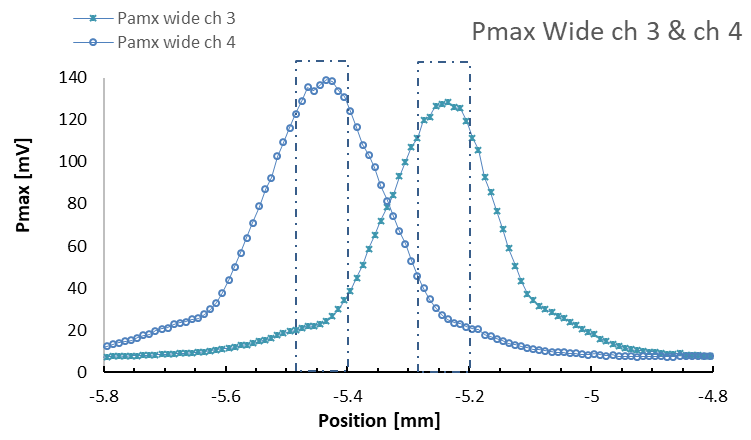}
\caption{Left: prototype BNL AC-LGAD strip sensor with 80\,$\mu$m wide strips and pitch of (left to right) 100, 150, 200\,$\mu$m. Right: sensor response ($P_{max}$) as a function of position (perpendicular to the strip) of two strips with 200~$\mu m$ of pitch~\cite{ACLGADpico}. The dashed lines highlight the position of the two strips in the plot. Data taken at the FNAL 120\,GeV proton test beam facility.}
\label{fig:FNAL_data}
\end{figure}

 The position resolution is calculated from the signal fraction as function of position between adjacent strips: 

\begin{equation}
    \label{Pos_resolution}
    \sigma(pos) = \sqrt{2} \frac{d(\textrm{Position})}{d(\textrm{Fraction})}\left(\frac{S}{N}\right)^{-1}
\end{equation}

The position resolution perpendicular to the strips for the studied 200\,$\mu$m pitch is 5--15\,$\mu$m across the sensor, a few \% of the pitch as seen in Fig.~\ref{fig:BNL_resolution}.

\begin{figure}[htbp]
\centering
\includegraphics[width=0.9\textwidth]{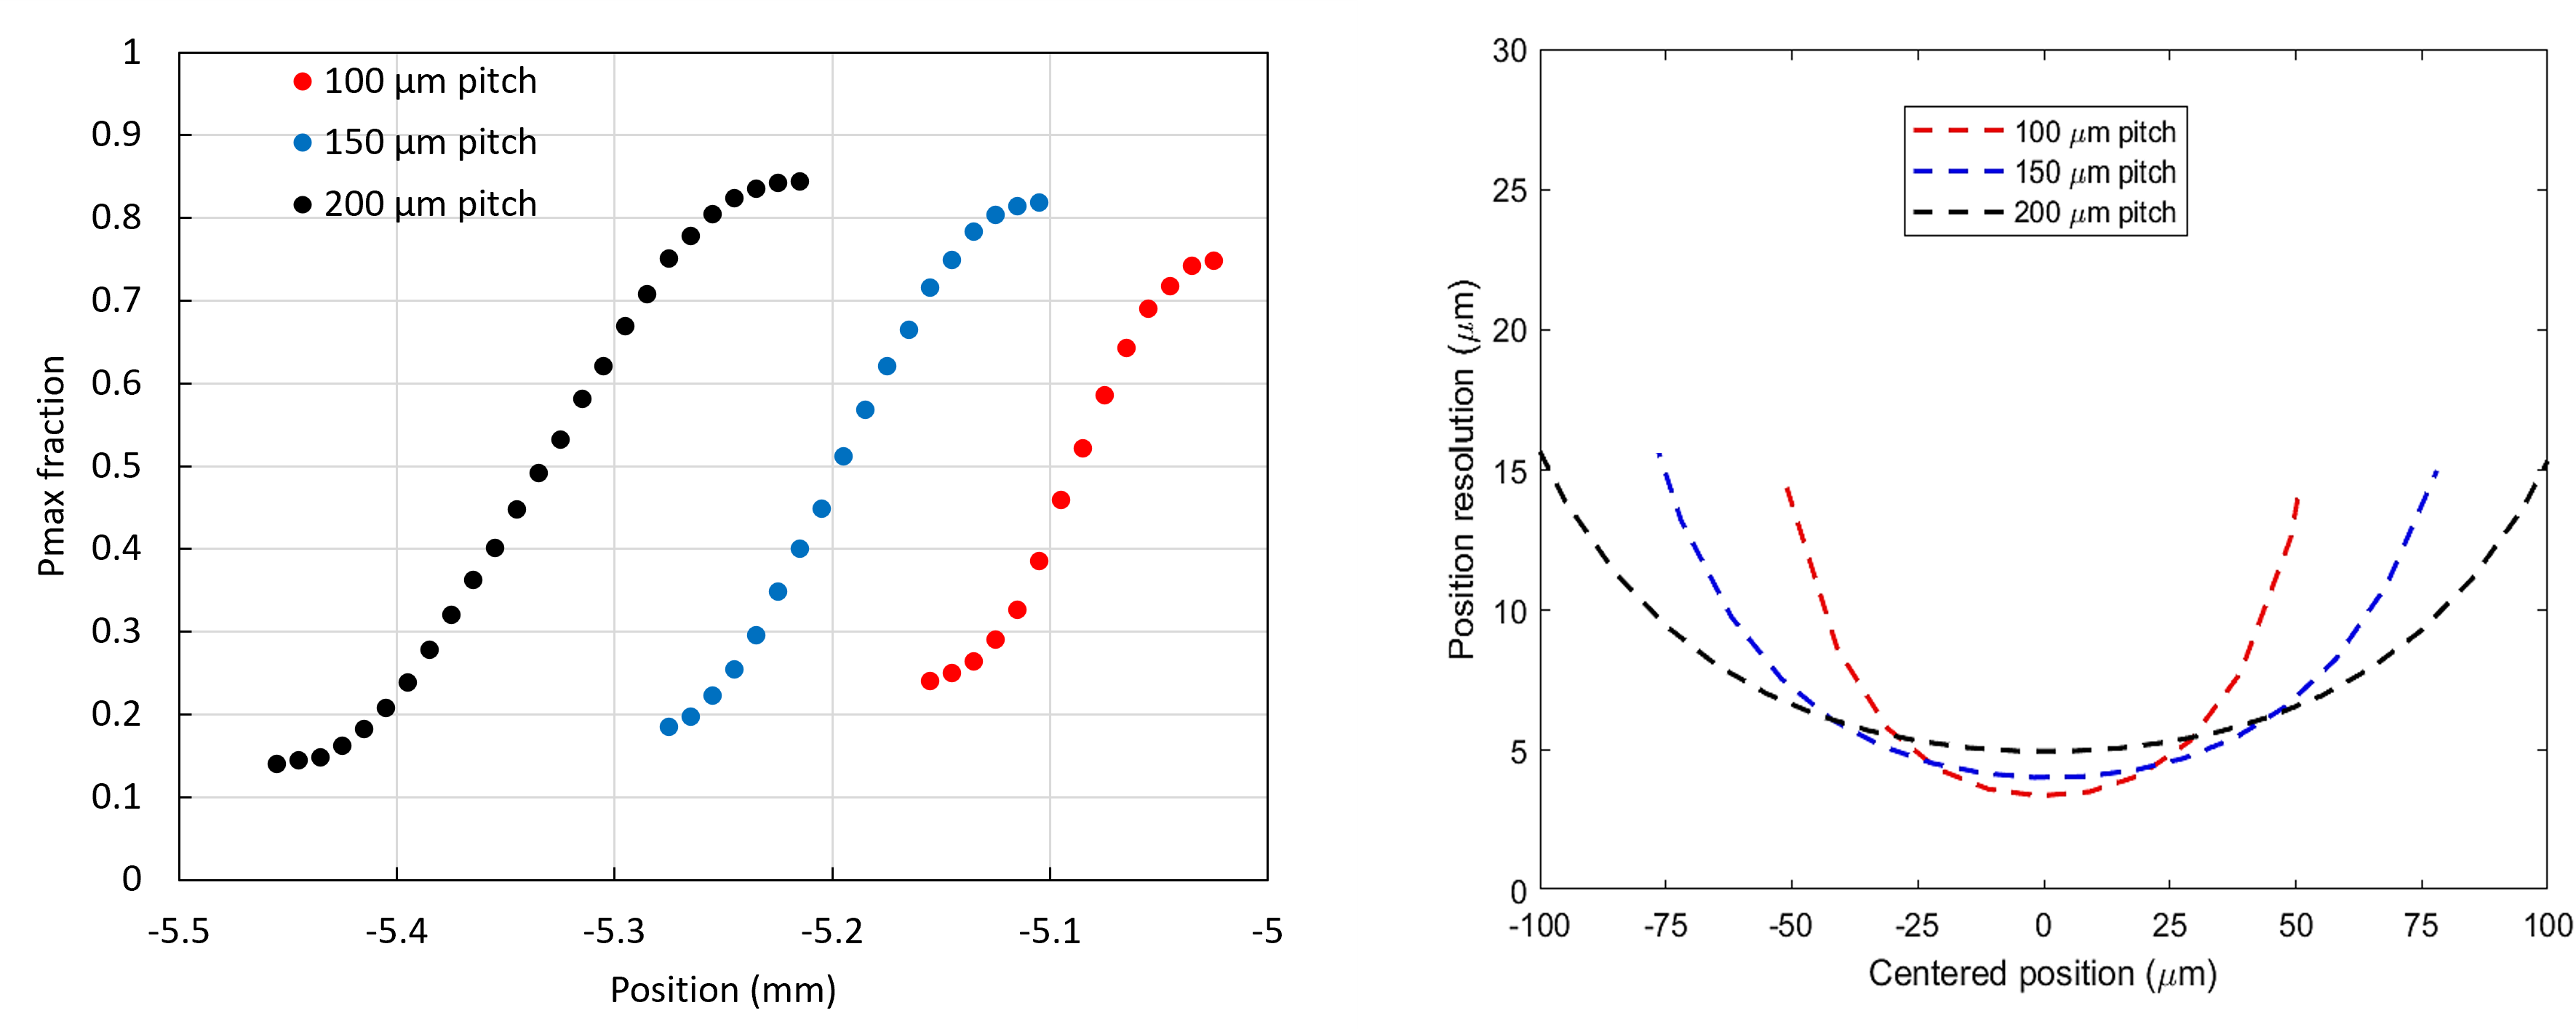}
\caption{Signal charge sharing and position resolution of AC-LGAD strip sensors fabricated by BNL, assuming a constant S/N of 60. Left: fraction of the maximum signal amplitude ($P_{max}$) measured in one channel with respect to the summed signal of two neighboring strips. Data taken at the FNAL 120\,GeV proton test beam facility. %Saturation at the center of the strips is observed, governed by the strip pitch. 
Right: position resolution over the respective strip pitch, determined with Eq.~\ref{Pos_resolution}. The zero point is in the middle of the gap between two strips. 
%Position resolution of 6 um and below can be achieved between strips, and even at the center of the metal strips, the position resolution remains at ca. 15 um for all pitches.
}
\label{fig:BNL_resolution}
\end{figure}

Strips were tested with readout connected at both ends, for this particular configuration the signal is additionally split between the two ends of the strip.
By applying the same fractional method of charge sharing, it is possible to reconstruct the hit position also in the direction parallel to the strip, as seen in Fig.~\ref{fig:double_side} (Left). 
A precision of a few hundred $\mu$m was found with a 2\,mm strips, giving a position resolution of 10\% of the strip length.
Having a double-connection readout setup would be more challenging in terms of mechanics, but would allow X-Y charge deposition reconstruction.

The envisioned metal size for the 200\,$\mu$m pitch strips, as well as other parameters of interest for the sensor such as the doping profile, needs to be confirmed after a testing R\&D campaign and TCAD simulations as shown in Appendix~\ref{sec:TCAD_app}.
In addition, some non-typical detector setup configurations, such as zig-zag strips, can be explored to identify muons traveling parallel to a strip, schematic shown in Fig.~\ref{fig:double_side} (Right).

\begin{figure}[htbp]
\centering
\includegraphics[width=0.5\textwidth]{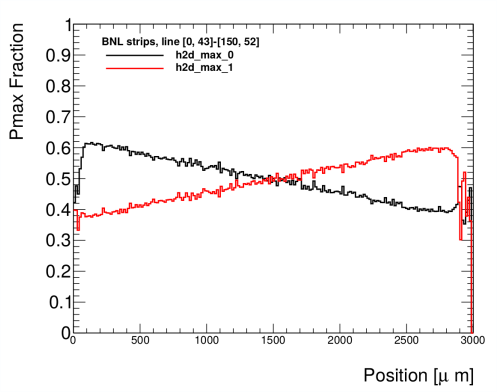}
\includegraphics[width=0.3\textwidth]{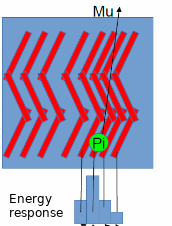}
\caption{Left: response of an AC-LGAD strip read out from both sides. Right: muon escaping parallet to the strip direction detected with zig zag strip geometry.}
\label{fig:double_side}
\end{figure}

As already stated, a dynamic range from MIP (positron) to several MeV (pion/muon) of deposited charge is expected in the ATAR. 
%For this reason the response of prototype sensors to high charge deposition has to be studied.
High ionizing events might affect the charge sharing mechanism, inducing charge also in electrodes far away from the charge deposition.
Since the event reconstruction relies on temporal pulse separation, the response to successive MiP and high charge deposition have to be studied \cite{Pulserep}.
Furthermore the effect of gain suppression for large charge deposition in LGADs has to be taken into account \cite{gainsuppr}.
To study these effects a test beam will be organized at the ion beam line of the University of Washington (CENPA) in 2022 to study the response of the aforementioned sensors to high ionizing events. 
Furthermore, laboratory tests will be conducted with an alpha source.

\subsection{TI-LGAD preliminary studies}
\label{sec:TILGAD_app}
Trench Isolated (TI) LGADs are a novel silicon sensor technology that utilizes a deep narrow trench to electrically isolate neighboring pixels to prevent breakdown, as opposed to standard LGADs which use a junction termination extension to prevent breakdown at the pixel edges \cite{9081916}. By utilizing the deep trench isolation technology, the no-gain region is reduced to a few micrometers, thus achieving a higher fill factor than regular LGADs. %, which is dependent on the fraction of the active sensor area with gain.
%If the inter-pad width from 50-100 $\mu$m, that of a standard LGAD, down to less than 10 $\mu$m, the fill factor naturally increases and allows for lower pitch.
The studies shown here were done on strip TI-LGADs sensors from Fondazione Bruno Kessler (FBK) \cite{9081916}. These strip sensors had a pitch of 100\,$\mu$m and had varied characteristics such as contact type, pixel border version, and one or two trenches.
The sensors have been tested using a laser TCT station, the setup is as described in Appendix~\ref{sec:ACLGAD_app}.
%with the exception that sensors are mounted on a LANL designed board with the same characteristics as the FNAL board. 

\begin{figure}[htbp]
\centering
\includegraphics[width=0.95\textwidth]{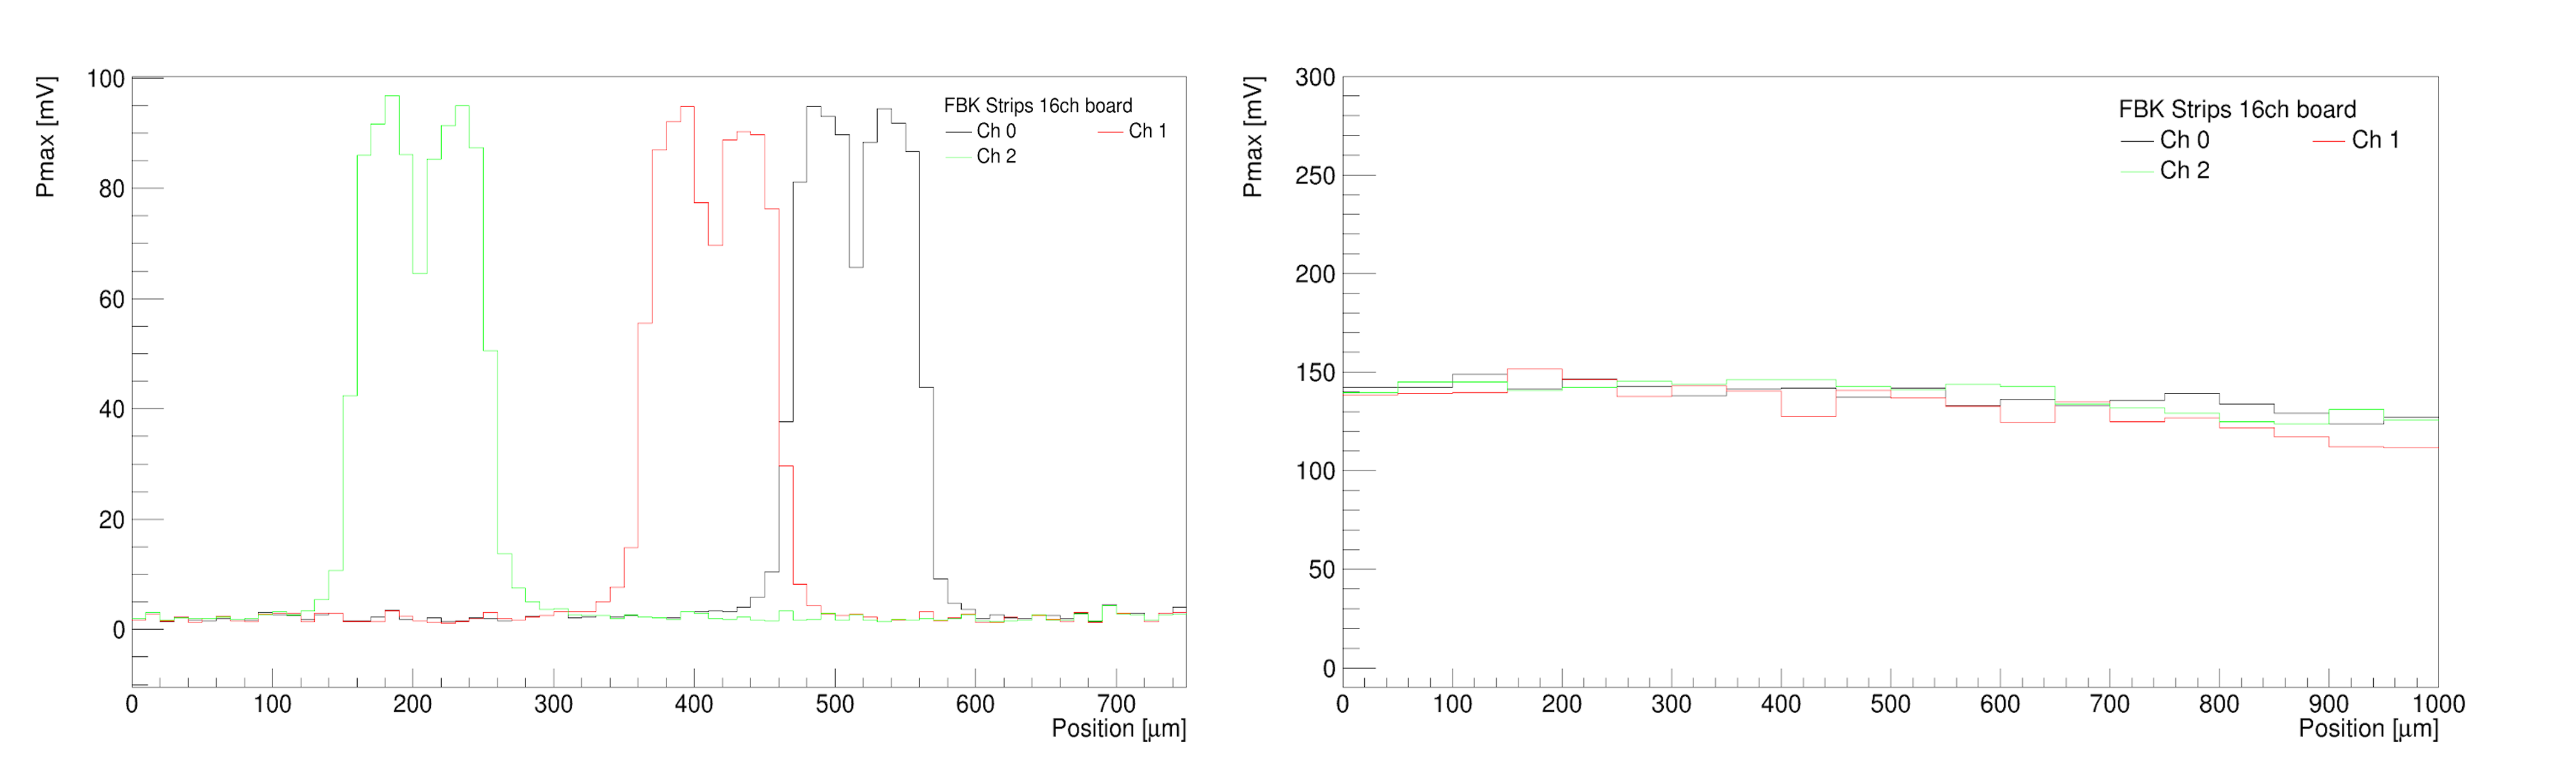}
\caption{Left: $P_{max}$ vs position across the strips is plotted. Ch0, Ch1, Ch2 correspond to the different strips being read out. There is minimal amount of “cross-talk” between neighboring strips. Right: $P_{max}$ vs position along the strip is plotted. The response across the different strips remains constant along the strip.}
\label{fig:TILGAD_data1}
\end{figure}

The response of the sensor as a function of position can be observed in Fig.~\ref{fig:TILGAD_data1}. On Fig.~\ref{fig:TILGAD_data1} Left, $P_{max}$, a measure of charge collection, is plotted on the y-axis versus the position going across different strips being read out on the x-axis. It can be seen that the no-gain region between two adjacent strips (red and black in the plot) is less than 10\,$\mu$m.
The sensor has the standard response of a conventional LGAD and exhibits a small amount of “cross-talk”. Figure~\ref{fig:TILGAD_data1} Right, shows the response of the sensor is constant along the strip. The sensor is mounted at an angle with respect to the IR laser so the fall-off of the response is expected to slightly decrease as the laser scans for larger distances along the strip. 

The measured signal across a TI-LGAD strip sensor is shown in Fig.~\ref{fig:TILGAD_data2}. The red pulse corresponds to a region of strong signal being for the strip being read out in channel 1 on the oscilloscope. The remaining signals (black and green) correspond to the position of the nearest strip being read out. The maximum values for the nearest strips correspond to ~3$\%$ of the maximum value of the red pulse showing there is good isolation between strips.

\begin{figure}[htbp]
\centering
\includegraphics[width=0.95\textwidth]{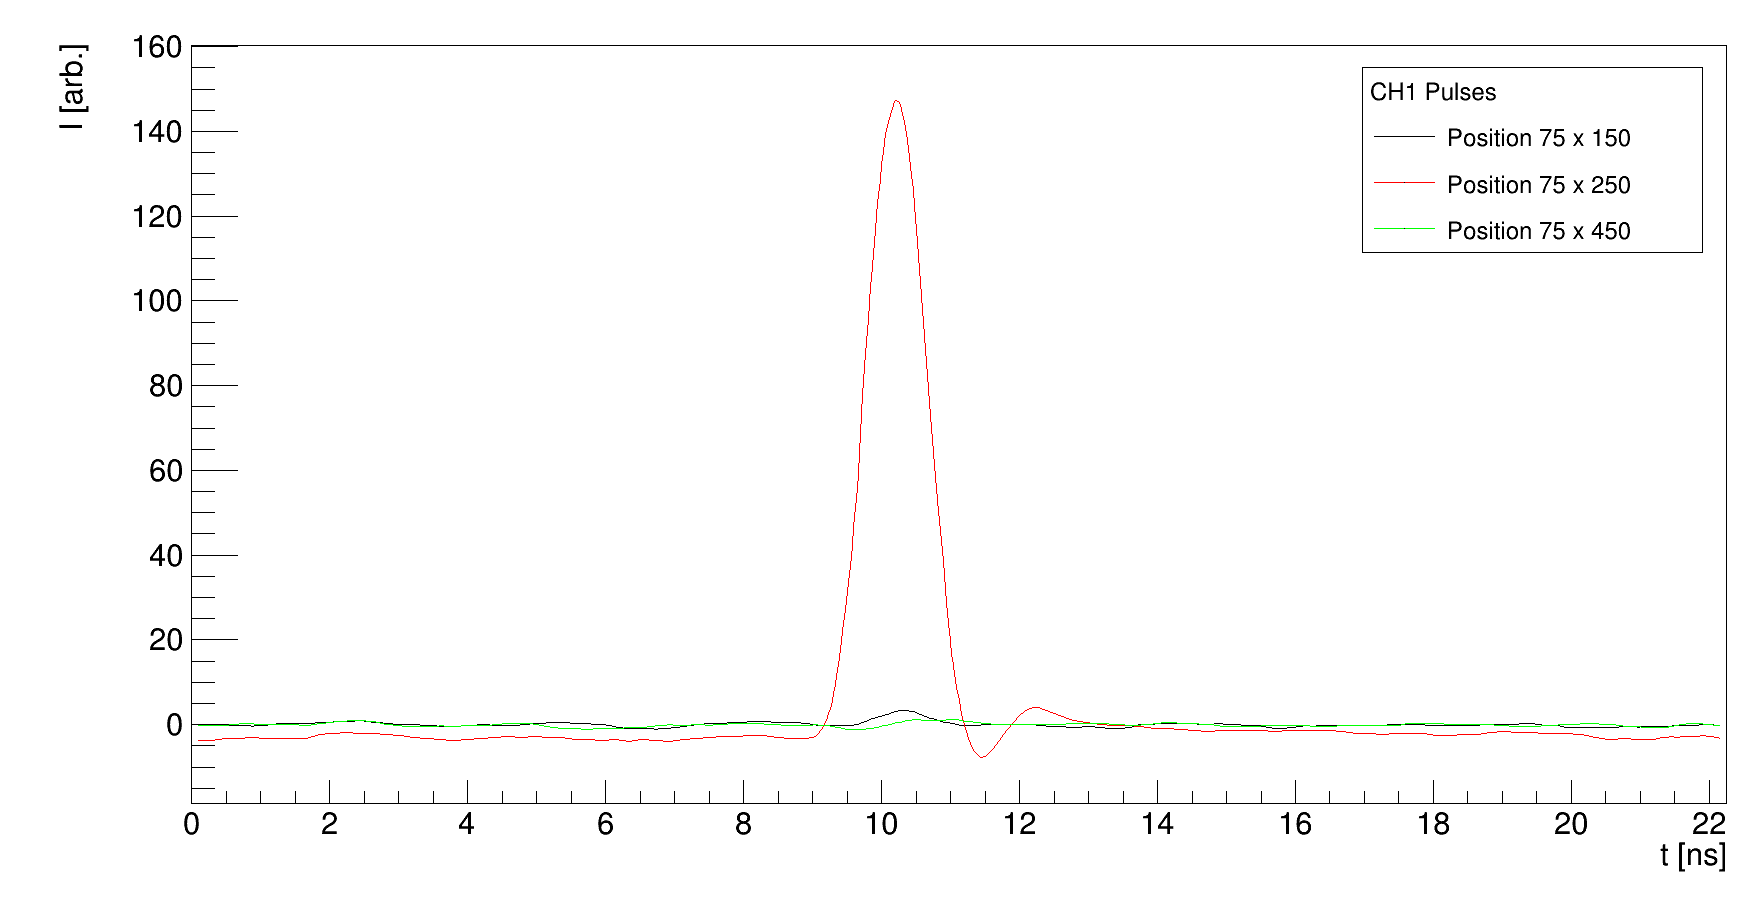}
\caption{Signals across a TI-LGAD strip sensor. The red pulse corresponds to a region of strong signal for the strip being read out. The black and red signals correspond to the position of the nearest strips. It can be observed there is “little” pickup from neighboring strips.}
\label{fig:TILGAD_data2}
\end{figure}

%%%%%%%%%%%%%%%%%%%%%%%%%%%%%%%%%%%%%%%%%%%

\subsection{TCAD simulation}
\label{sec:TCAD_app}
AC-LGADs have several parameters that can be tuned to optimize the sensor response to the specific application.
The geometry of the electrodes in terms of pitch and pad dimension is the most important one, however also the N+ sheet resistivity and the dielectric thickness between N+ and electrodes influence the charge sharing mechanism.
These parameters have been studied with the TCAD Silvaco \cite{Silvaco} to have a good representation of the observed sensor performance. Simulations with TCAD software are important to compare with existing prototype data and to help in optimizing the design. 

Figure~\ref{fig:simulation} (Left) shows the simulated waveforms of four metal pads using TCAD Silvaco The sensor is a 200\,$\mu$m pitch strip sensors with N+ sheet resistivity of 500\,$\Omega$. 
Figure~\ref{fig:simulation} (Right) is the Pmax profile of 200\,$\mu$m pitch strip sensors with different sheet resistivity and the same geometry of the BNL strip prototype already introduced.
500\,$\Omega$ shows a reasonably good match with FNAL TB data from Fig.~\ref{fig:FNAL_data}, Right. 
These simulations are for 50\,$\mu$m thick sensors, to simulate the final PIONEER prototype they need to be redone for 120\,$\mu$m of thickness.
The calibrated simulation will be used as input to prototype productions to optimize the sensor design for the PIONEER specific application.

\begin{figure}[htbp]
\centering
\includegraphics[width=0.4\textwidth]{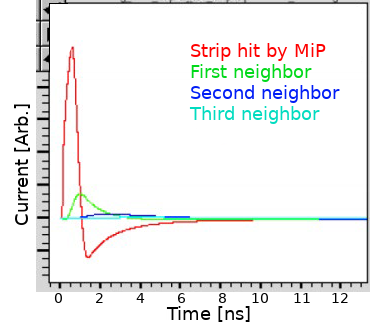}
\includegraphics[width=0.55\textwidth]{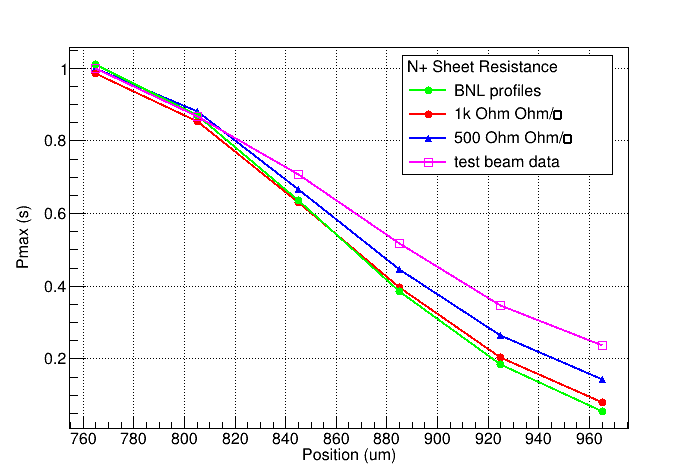}
\caption{Left: AC-LGAD strip simulated waveform with TCAD Silvaco, charge deposition is the strip with the red waveform, green is first neighbor, blue is second neighbor. Right: Pulse maximum (normalized) as a function of position for a strip with 80\,$\mu$m width and 200\,$\mu$m pitch. Left edge of the plot is the center of the readout strip. Curves are for data (FNAL testbeam) and TCAD Silvaco simulation with several N+ sheet resistivity. }
\label{fig:simulation}
\end{figure}

%%%%%%%%%%%%%%%%%%%%%%%%%%%%%%%%%%%%%%%%%%%

\subsection{Electronics and readout chain}
\label{sec:ATAR_electronics_app}

To read out the ATAR sensors, two crucial electronic components need to be identified: an amplifier chip and a digitizer board.
%The ASIC sits on the flex connected to the sensor with several centimeters of separation.
The ASIC needs to be fast enough for the sensor in use; for the signal rise time in the 120\,$\mu$m-thick prototype sensors,  a bandwidth of 1\,GHz should be sufficient.
However, the high dynamic range (2000) requirement for the ATAR brings major complications to the readout.
Current fast readout chips usually have a dynamic range of $<$~1000, since they are targeted at MIPs-only detection in tracker sub-systems.
One possibility is to develop an amplifier chip with logarithmic response as well as a high enough bandwidth, currently no such chip exists with the necessary characteristics.
Another alternative is to stream to the digitizer both the amplified (for MIP) and non-amplified (non-MIP) signals, or use two different amplifiers with different gains.
Yet another option is to adopt a chip capable of dynamic gain switching.
Nevertheless already available integrated chips, such as FAST~\cite{OLAVE2021164615} and FAST2, will be evaluated (Fig.~\ref{fig:FAST2}).
Some new ASIC technologies that are being developed at UCSC in collaboration with external companies can run with 2.5V maximum signal, this allows for an increased dynamic range.

\begin{figure}[htbp]
\centering
\includegraphics[width=0.45\textwidth]{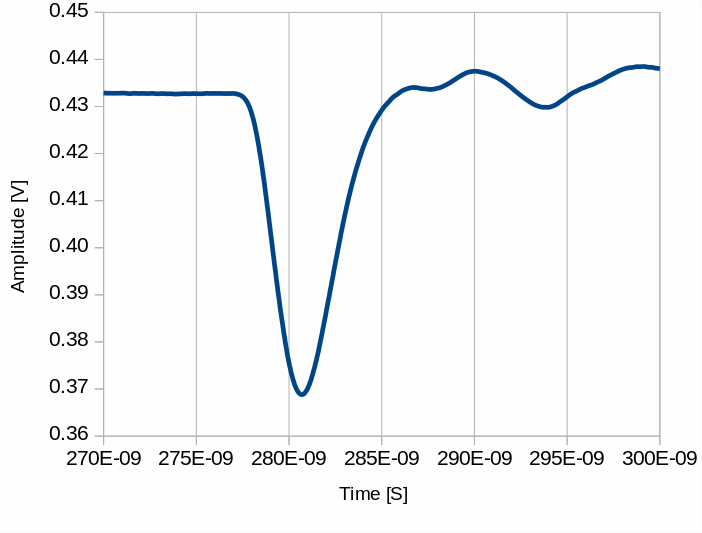}
\includegraphics[width=0.45\textwidth]{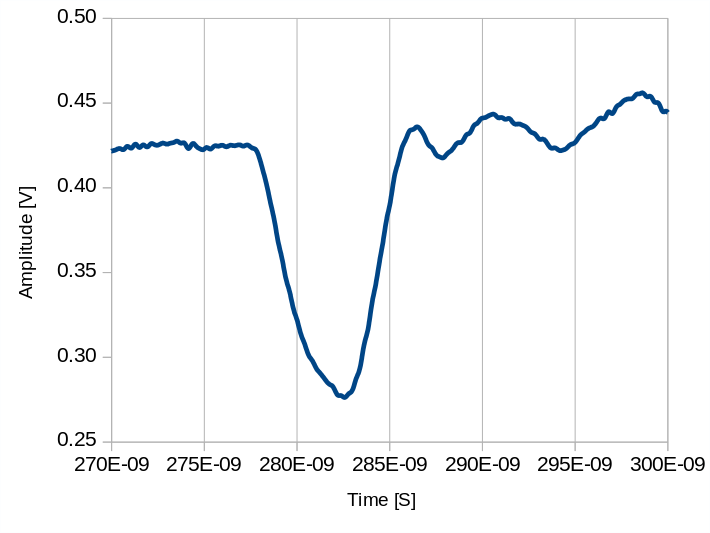}
\caption{Left: FAST2 analog calibration input response. Right: FAST2 analog saturated response, the pulse becomes wider and the peak flattens. In both cases the return to baseline is with a 5~ns time range.}
\label{fig:FAST2}
\end{figure}

To successfully reconstruct the decay chains, the ATAR is expected to be fully digitized at each event.
%, the fast charge collection time of thin LGADs will allow to separate subsequent charge depositions by using advanced deconvolution algorithms.
To achieve this goal, a high bandwidth digitizer with sufficient bandwidth and sampling rate have to be identified. 
The same issue afflicting the amplifier, the high dynamic range, is also problematic for the digitization stage. 
A digitizer that would suit PIONEER's requirements needs to be identified, a ready commercial solution would be the best option but the cost per channel might be prohibitive. 
For this reason the collaboration is exploring the possibility to develop a new kind of digitizer specific to this application.

Since the amplification chip has to be positioned away from the active region, the effect of placing a short (5\,cm) flex cable between the sensor and the amplification stage has to be studied.
The high S/N provided by LGADs would allow the signal to travel without compromising the transmitted information.
A prototype flex was produced (Fig.~\ref{fig:flex}) and the effect on LGAD signals will be studied.

\begin{figure}[htbp]
\centering
\includegraphics[width=0.45\textwidth]{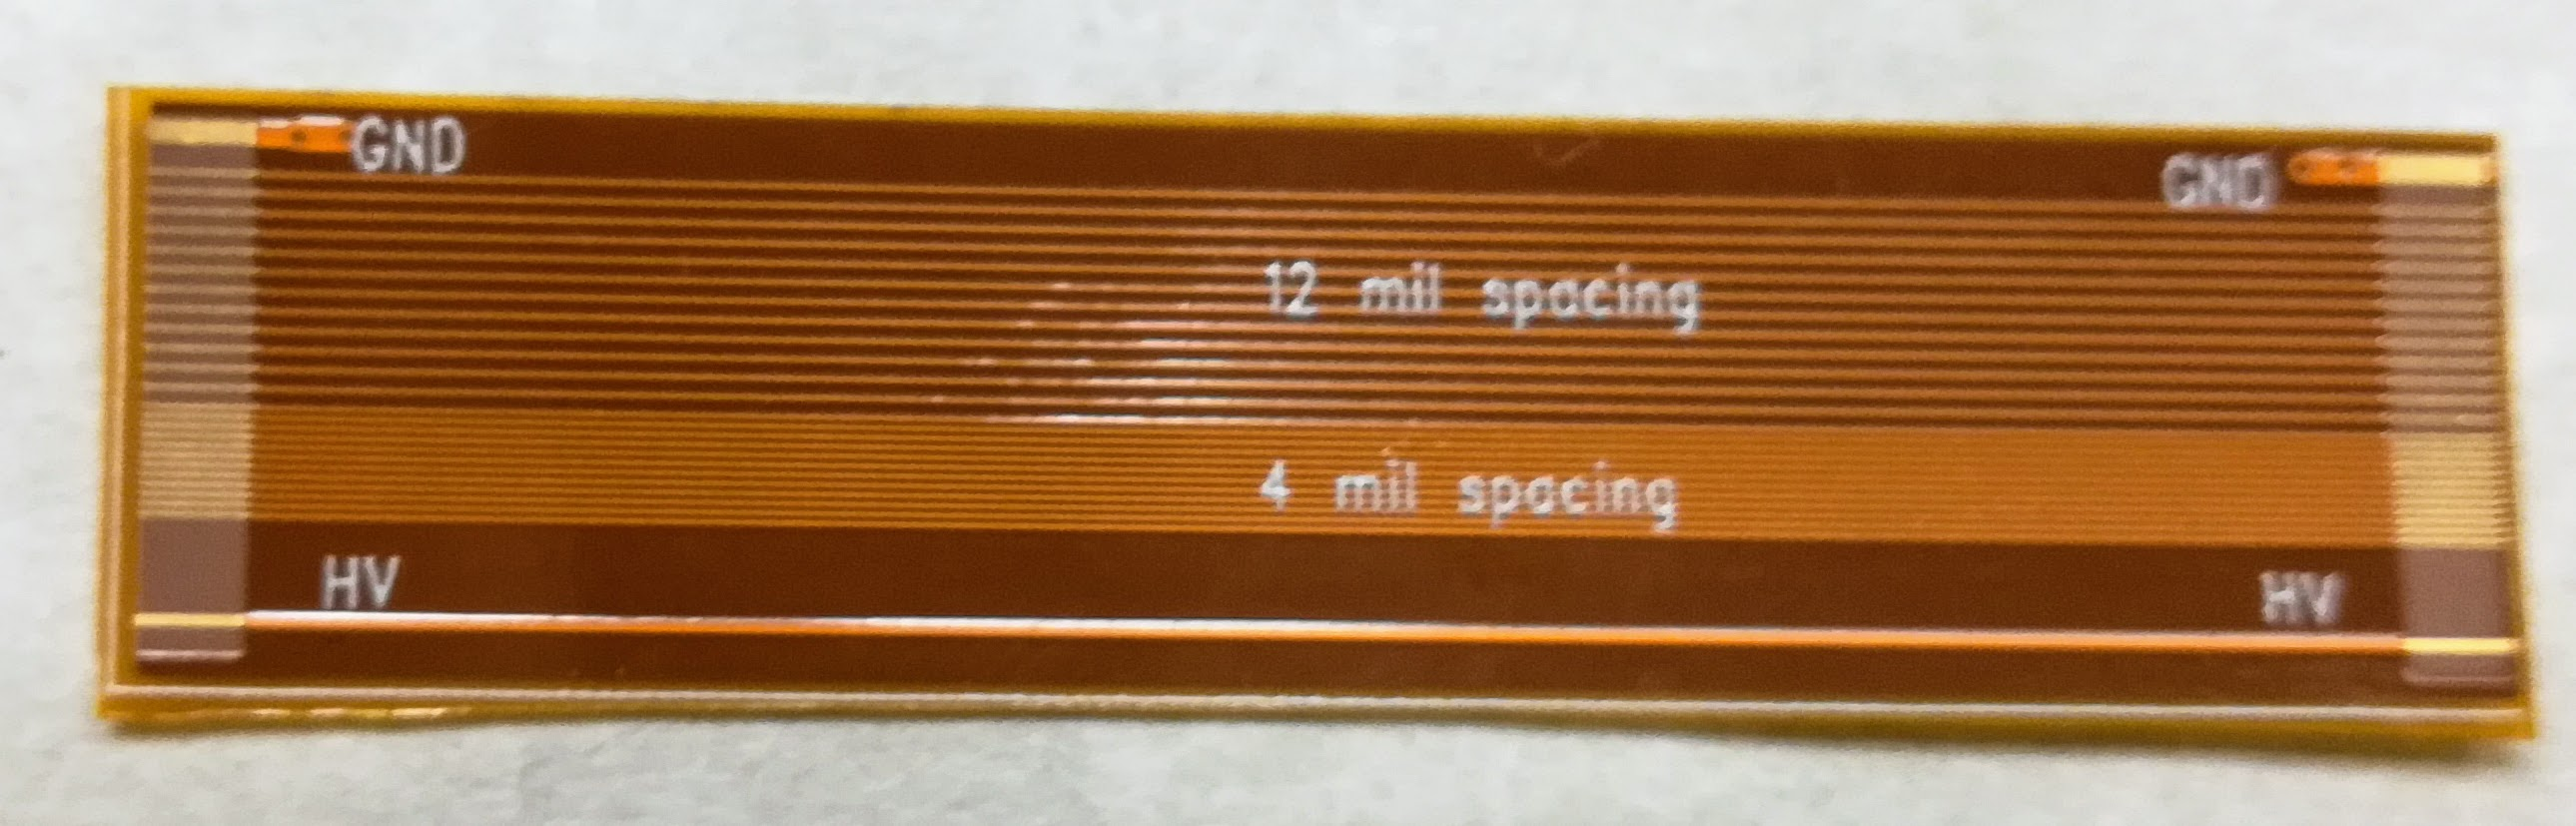}
\caption{Picture of prototype flex cables with difference trace separations.}
\label{fig:flex}
\end{figure}

%%%%%%%%%%%%%%%%%%%%%%%%%%%%%%%%%%%%%%%%%%%

\subsection{Mechanics}
\label{sec:ATAR_mech_app}
The ATAR mechanical support needs to introduce as little dead material as possible to avoid degradation of the positron energy. 
The wirebonds between the sensor and the flex are theoretically strong enough to hold the sensor, however additional support is necessary.
Figure~\ref{fig:mechanics} (Left) show the tentative U-shaped sensor support with 4 connection at the corners; the open side of the support is for flex connection. 
Four staves at the corners would align the planes and hold them together.
Further, the entire ATAR structure is supported by a stave coming from the back plane.
On the HV side the chip are directly connected, on the strip side an interposer layer (Kapton) between chips avoids shorting between strips.
The materials for the support can be carbon fiber or Pyrolytic graphite, providing low density and heat conductivity.
The flex on the chip side can be supported in several ways:
\begin{itemize}
    \item Extruding support from the U-shaped sensor support
    \item Flex can be bent and glued on the side of the sensor
    \item Thin kapton layer extruding from the flex glued on the back of the sensor
\end{itemize}
On the other side the flex is connected to the back support and connected to the interposer board between two flexes. Figure~\ref{fig:mechanics} (Right) shows the mechanical support.
The second flex runs to the back crate with the digitizers.

\begin{figure}[htbp]
\centering
\includegraphics[width=0.45\textwidth]{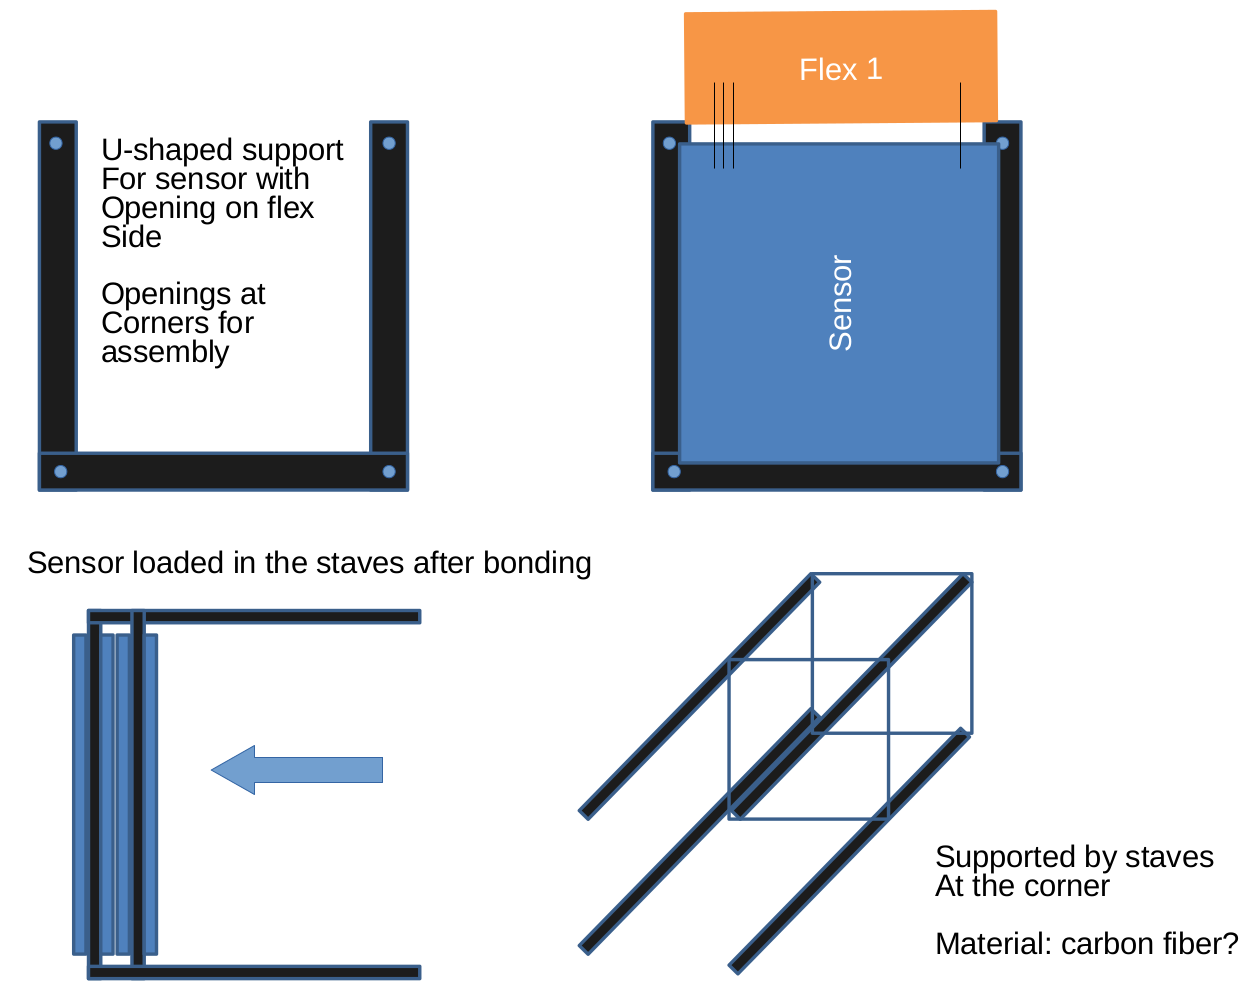}
\includegraphics[width=0.45\textwidth]{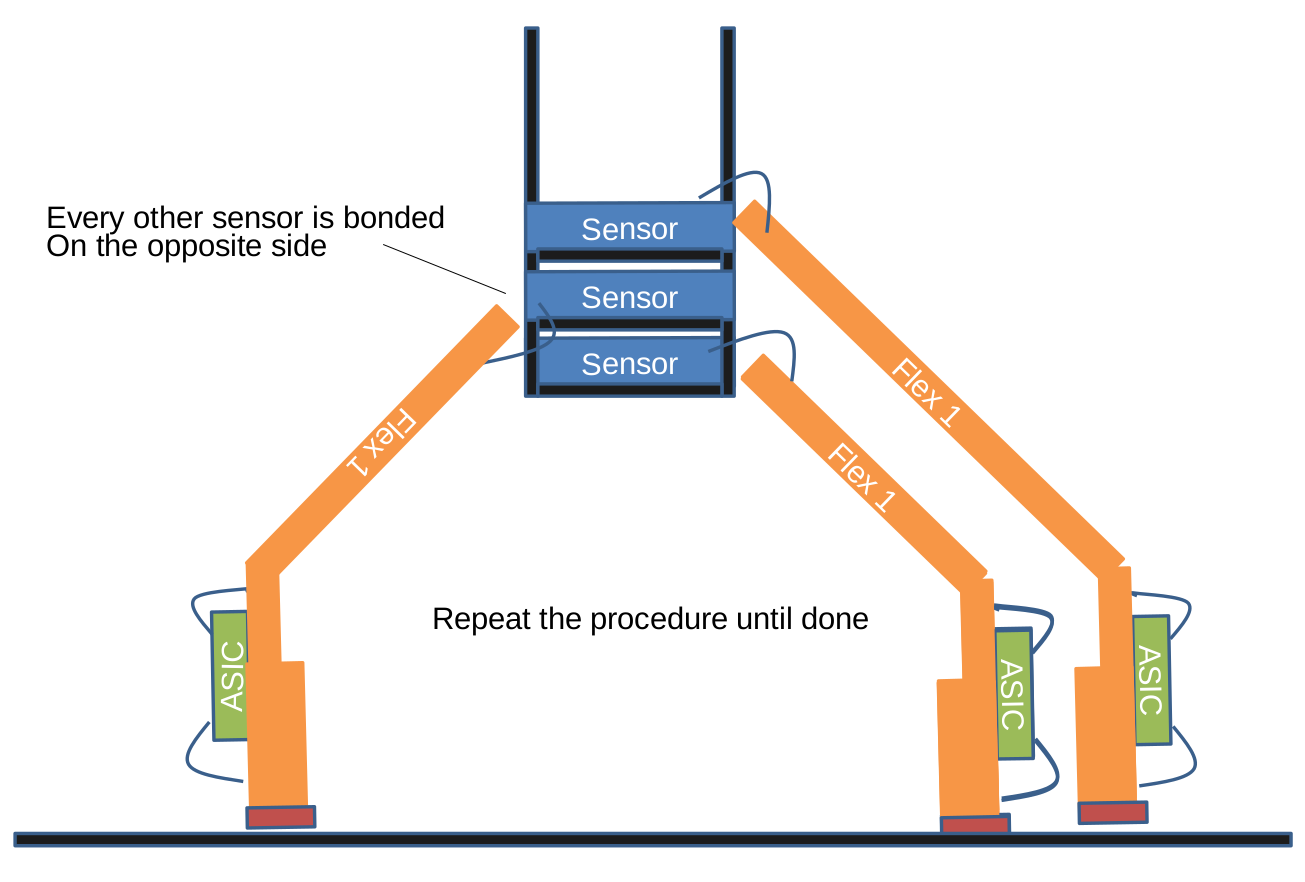}
\caption{Left: U-shaped support and staves. Right: final mechanic support assembled.}
\label{fig:mechanics}
\end{figure}

A tentative mounting procedure for the ATAR is as follows:
\begin{itemize}
    \item Glue ASIC to flex, wire bond the connections
    \item Connect flex to sensor via wire bonds
    \item Glue sensor to support 
    \item Slide support in staves while using a temporary flex support
    \item Slide all sensor modules in the staves
    \item Remove temporary support, bend wire bonds and flex, then connect to back wheel
\end{itemize}

Another issue to take into account is the thermal load of the sensors.
Before irradiation sensors will likely run at 300~V -- with ~nA current through each of 50 sensor layers, the total power dissipation would be a few tens of $\mu$W for the entire ATAR. This load can likely be extracted with the U-shape supports and staves. If needed, air flow can be enhanced to increase the heat extraction. 
After irradiation the current and the voltage will increase due to radiation damage, but this is not a concern for the PieNU phase.
For the entire PieNU+PiBeta the sensors will likely reach 600V, with $\mu$A current multiplied by 50 and thus a total power dissipation of tens of mW (based on \cite{CERN-LHCC-2020-007}), i.e. a factor of 1000 higher than during initial operation. This might be problematic, but a simple solution would be the substitution of the ATAR at the mid-life of the experiment.

%%%%%%%%%%%%%%%%%%%%%%%%%%%%%%%%%%%%%%%%%%%

\subsection{Alternative designs}
\label{sec:ATAR_designs}
A few alternative designs for the ATAR can be considered:
\begin{itemize}
    \item Use of thinner sensors (50\,$\mu$m) with pairs of sensors with same direction of strips, so that they would be read out by a single flex per pair. This would double the granularity in Z (although the X-Y information will not be provided at alternating planes) without doubling the number of flexes.
    \item In the central part of the ATAR read out, double-sided strips to have X-Y tracking.
    \item Using 8 instead of 4 angles for the sensors, strips are rotated 45 degrees each plane, giving more space to exiting flexes.
    \item Instead of ATAR with positron tracker and degrader, construct an improved ATAR that does full tracking. To achieve this, different sensor thickness would be used depending on the position.
\end{itemize}

%%%%%%%%%%%%%%%%%%%%%%%%%%%%%%%%%%%%%%%%%%%

\subsection{LGAD energy resolution}
\label{sec:LGAD_energy_app}
Preliminary data taken at the Stanford Light source (SSRL) \cite{GALLOWAY20195} show that LGADs can detect low energy X-rays with a reasonable energy resolution (8\% to 15\%) thanks to the internal gain.
The beamline at SSRL had a 2\,ns repetition rate and single pulses were completely separated with 50\,$\mu$m thick LGADs.
Figure~\ref{fig:energy} shows some results of detection of X-rays with LGADs.

\begin{figure}[htbp]
\centering
\includegraphics[width=0.45\textwidth]{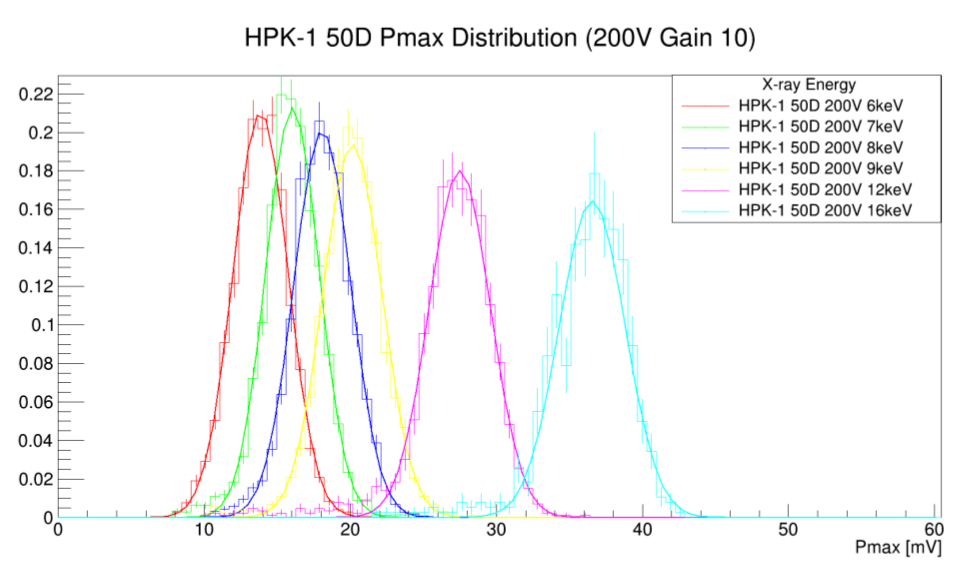}
\includegraphics[width=0.45\textwidth]{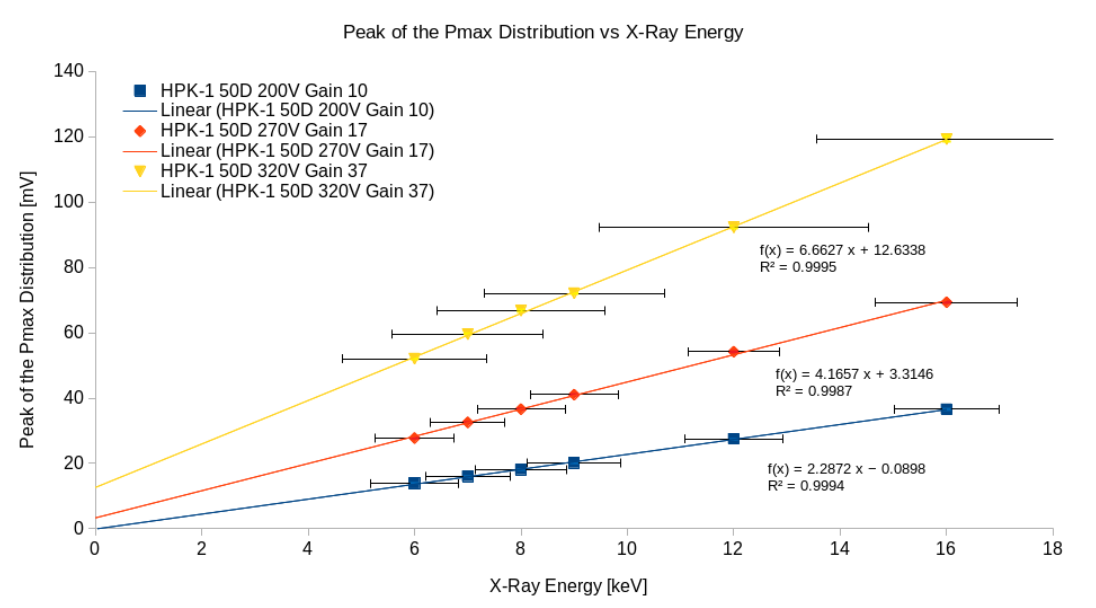}\\
\includegraphics[width=0.45\textwidth]{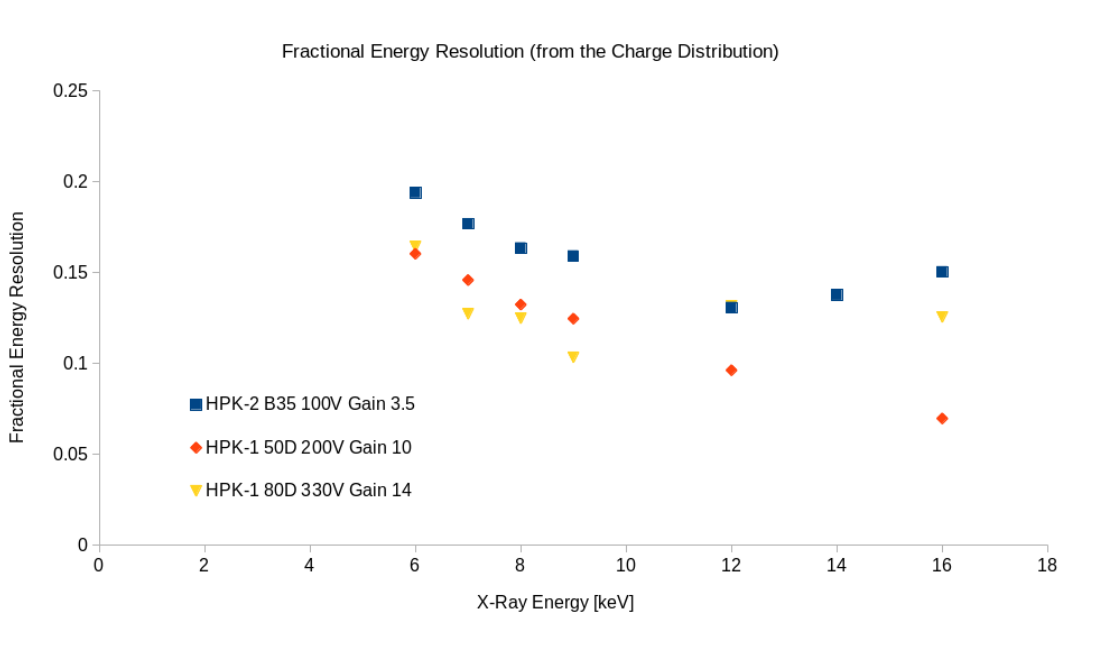}
\caption{Top-Left: Event distribution of pulse maximum for different X-ray energy, data is for a HPK 50~$\mu$m LGAD at gain 10. Top-Right: Peak of the pulse maximum distribution vs X-ray energy, data is for a HPK 50~$\mu$m LGAD at different gain levels. Bottom: Fractional energy resolution as a function of X-ray energy, data is for three HPK LGADs of 35~$\mu$m, 50~$\mu$m and 80~$\mu$m of thickness. }
\label{fig:energy}
\end{figure}

%%%%%%%%%%%%%%%%%%%%%%%%%%%%%%%%%%%%%%%%%%%

\subsection{ATAR timeline}
\label{sec:ATAR_timeline_app}
PIONEER is set to start taking data on a timescale of 7 years at PSI (see Sec.~\ref{sec:timeline_estimate}), the ATAR is a small project in terms of production (roughly 0.01~m$^2$ of sensor area) but still requires significant R\&D for sensors, electronics, digitization and mechanics. An envisioned path forward for this project is the following:
\begin{itemize}
    \item Sensor characterization and design optimization is the top priority, so the first interest is to continue the collaboration with Brookhaven National Laboratory in the development of AC-LGAD and DJ-LGAD prototypes. This will culminate in a PIONEER-specific prototype production that should happen within 2 years from now. To steer the design effort, simulations are crucial. At UCSC, TCAD (Silvaco and Sentaurus) simulation experts are setting up a reliable simulation of the available AC-LGAD prototypes. At the same time TI-LGADs produced by FBK will be fully evaluated as an alternative.
    \item Having the amplifier chip several cm away from the LGAD sensor is rather unconventional and the effect on the response needs to be understood; a first connection flex prototype was produced and will be thoroughly tested within 2023. Likely a second flex production with the lesson learned will happen in the same year.
    \item A crucial aspect to understand is the energy resolution of LGAD devices (which was never studied thoroughly by the community since it is not of interest for common HEP applications) as well as the gain suppression mechanism~\cite{gainsuppr}. UCSC is currently collaborating with the University of Washington to organize a test beam at the the ion beam line of CENPA to study the response of LGADs to high ionizing events. This will tentatively happen in Q2/Q3 2022 with already available sensor prototypes and analog amplifier boards.
    \item Building of a first ATAR demonstrator (ATAR0) with available sensor prototypes: the current BNL AC-LGAD production has 2.5~cm long strips with a pitch of 500~$\mu$m, which is close to the final 200~$\mu$m 2x2~cm$^2$ ATAR design (however the sensor thickness is 50~$\mu$m instead of the final design 120~$\mu$m). Since a 50~$\mu$m thick sensor is fabricated on a support wafer of a few 100s $\mu$m, the devices would need to undergo an etching procedure to have full active volume, the thinning procedure can be executed at BNL. The BNL sensor group has experience with wafer lapping and chemical mechanical planarization (CMP). The sensor would be initially lapped to remove most of the thickness of the handling thick substrate, followed by CMP for final polish. The etching rate would be determined on dummy wafers and the process would be optimized to reach the required final thickness.
    The prototype would have a few layers (5-10) with a reduced number of channels to detect the temporal development of a muon or pion decay. As the layers would need to be very close to each other, a suitable readout board needs to be developed. The board might be built with discrete components or using a chip such as FAST2.
    The prototype would be then tested in a pion/muon beamline either at TRIUMF or a PSI. Hopefully such a prototype can be produced by the end of 2023.
    \item Identification of a suitable chip for the analog amplification; the ideal path would be to find an already existing chip (FAST2) and characterize it with LGAD sensors similar to what would eventually be used in the ATAR. In parallel an effort to produce a new chip can be pursued through external companies (SBIR-like funding). A prototype readout chip needs to be ready by 2024.
    \item Identification of a digitizer chip: currently available digitizers such as DRS4 are too expensive for the number of channels in the ATAR. Furthermore a complicated triggering system might be needed for AC-LGAD readout. Small companies might be available to develop a new chip with the needed performance by modifying existing designs. A suitable digitizer chip needs to be identified/developed by 2024.
    \item The support mechanics and thermal transport calculation needs to be studied well for the success of the ATAR. A discussion is ongoing between technicians from UCSC and UW for the design of the mechanic support and mounting procedure. Thermal load tests can be conducted with an ATAR mock-up made with Silicon heaters, thermal calculations are also foreseen.
\end{itemize}

\clearpage
